# Supplementary material for: FlowShield: cryptocurrency anti-money laundering with transaction semantics parsing and fund flow tracking
Source: arXiv:2608.17355 source file (2026-08-18)
Supplement: Supplementary file 1 [file additional_text.tex]

This flow has reached an unprecedented economic scale; in 2025 alone, illicit cryptocurrency volumes reached record highs, with approximately USD 158 billion in value moving through various obfuscation pipelines \cite{chainalysis2025}. While illicit activity often constitutes a small fraction of total on-chain volume, the concentration of these funds in professionalized laundering-as-a-service (LaaS) networks, such as Chinese-language money laundering ecosystems (CMLNs), which processed an estimated USD 16.1 billion in 2025, poses a systemic risk to market integrity \cite{chainalysis2026cmln, bis_bulletin_111}. These ecosystems operate through distinct service typologies, ranging from ``running point'' brokers who act as initial entry channels to ``money mule motorcades'' that execute complex layering schemes via networks of rented bank accounts and digital wallets. A prominent mechanism within this economy is the ``Black U'' service, where vendors purchase illicit stablecoins (like USDT) at a discount and utilize automated swapping infrastructure to clear large transactions \cite{chainalysis2026cmln, chainalysis2025}. To mitigate counterparty risk in this underground market, these vendors often operate on ``guarantee platforms'' like Huione, which function as illicit escrow services to insure transactions between criminals.

For financial institutions and Virtual Asset Service Providers (VASPs), this professionalization has resulted in a staggering compliance burden. Global financial crime compliance costs have surged, driven by intensified regulatory scrutiny and the quadrupling of global financial penalties \cite{bis_bulletin_111, fatf2025targeted}. The operational challenge is exacerbated by ``alert fatigue,'' where existing rule-based anti-money laundering (AML) frameworks suffer from error rates as high as 95--99\%, mistakenly flagging legitimate accounts and creating massive operational waste \cite{bis_bulletin_111, kykynezhdy2024}. This inefficiency stems from a fundamental inability to manage the ``trace discontinuity'' inherent in modern laundering, where assets are fragmented across decentralized finance (DeFi) protocols and cross-chain bridges \cite{huo2025shedding, fu2025sok}.

Current regulatory frameworks face a critical ``sunrise issue,'' where the inconsistent implementation of global standards, such as the FATF Travel Rule, creates fragmented compliance environments that illicit actors actively exploit \cite{fatf2025targeted}. Significant gaps persist; a substantial number of jurisdictions have yet to implement basic VASP licensing or risk assessment regimes, allowing criminal networks to leverage ``jurisdictional arbitrage'' by routing funds through non-compliant offshore exchanges or regions with weak enforcement \cite{fatf2025targeted, dupuis2021money}. Furthermore, the traditional intermediary-based regulatory model is increasingly strained by DeFi, where regulators struggle to identify responsible entities (VASPs) within automated protocols, leaving vast portions of the ecosystem effectively unsupervised \cite{remolina2024defi, fatf2025targeted}. This disconnect is exacerbated by a ``regulatory dialectic,'' where static compliance frameworks fail to keep pace with illicit actors who rapidly adopt privacy-enhancing technologies, such as mixers and cross-chain bridges, to evade detection \cite{dupuis2021money, huo2025shedding, ofsi2025crypto}.

The defining trend of 2025, ``chain-hopping,'' illustrates this gap in real time. Large-scale security incidents, most notably the February 2025 Bybit heist involving the theft of approximately USD 1.5 billion in Ethereum, showcase how attackers use internal contract calls and cross-chain swaps to break traditional value-continuity boundaries \cite{ding2026bybit, huo2025shedding}. For the business sector, these ``fragmented trails'' represent more than a security risk; they capture vital liquidity and complicate the integration of digital assets into mainstream economic activity. Consequently, there is an urgent demand for ``semantics-aware'' and ``fund-flow-aware'' detection models that can provide the explainable forensic evidence required for institutional-grade compliance and global regulatory standards.
